# Supplementary material for: Representing Molecular Ground and Excited Vibrational Eigenstates with Nuclear Densities obtained from Semiclassical Initial Value Representation Molecular Dynamics
Source: arXiv:2012.03712 source file (2020-12-07)
Supplement: Supplementary file 1 [file Supplementary.pdf]

# SUPPLEMENTARY MATERIAL: Representing Molecular Ground and Excited Vibrational Eigenstates with Nuclear Densities obtained from Semiclassical Initial Value Representation Molecular Dynamics

Chiara Aieta
*Dipartimento di Chimica, Università degli Studi di Milano, via C. Golgi 19, 20133 Milano, Italy*

Gianluca Bertaina
*Dipartimento di Chimica, Università degli Studi di Milano, via C. Golgi 19, 20133 Milano, Italy and Istituto Nazionale di Ricerca Metrologica, Strada delle Cacce 91, 10135 Torino, Italy*

Marco Micciarelli
*Dipartimento di Chimica, Università degli Studi di Milano, via C. Golgi 19, 20133 Milano, Italy*[*]

Michele Ceotto
*Dipartimento di Chimica, Università degli Studi di Milano, via C. Golgi 19, 20133 Milano, Italy*[†]

We report the list of coefficients of the water vibrational wavefunctions, and additional plots of distributions of the protonated glycine molecule, useful to support the discussion in the main text. The ground state wavefunction expansion for protonated glycine were already reported in our previous study [C. Aieta et. al. Nat Commun 11, 4348 (2020)].

[*] marco.miccia@gmail.com
[†] michele.ceotto@unimi.it

## I. EXPANSION COEFFICIENTS FOR WATER MOLECULE EIGENFUNCTIONS

Table S1. Expansion coefficients for the ground state semiclassical eigenfunction of water.

$|e_0\rangle$

| $K_1$ | $K_2$ | $K_3$ | $C^{SC}_{0,\boldsymbol{K}}$ |
|---|---|---|---|
| 0 | 0 | 0 | 0.986265 |
| 1 | 0 | 0 | -0.161410 |
| 2 | 0 | 0 | 0.023172 |
| 1 | 0 | 2 | -0.015495 |
| 3 | 0 | 0 | -0.014678 |
| 0 | 0 | 2 | 0.009129 |
| 0 | 2 | 0 | 0.008690 |
| 0 | 1 | 0 | 0.004981 |
| 1 | 2 | 0 | 0.004192 |
| 2 | 0 | 2 | 0.003212 |
| 4 | 0 | 0 | 0.003152 |
| 0 | 1 | 2 | 0.002151 |
| 0 | 3 | 0 | -0.001890 |
| 0 | 2 | 2 | 0.001261 |
| 2 | 1 | 0 | 0.001094 |
| 0 | 0 | 4 | 0.001085 |

$|e_1\rangle$

| $K_1$ | $K_2$ | $K_3$ | $C^{SC}_{1,\boldsymbol{K}}$ |
|---|---|---|---|
| 0 | 1 | 0 | -0.988406 |
| 1 | 1 | 0 | 0.135606 |
| 0 | 2 | 0 | 0.044834 |
| 0 | 3 | 0 | -0.033905 |
| 2 | 1 | 0 | -0.020645 |
| 3 | 1 | 0 | 0.016937 |
| 1 | 1 | 2 | 0.014008 |
| 0 | 4 | 0 | 0.012612 |
| 1 | 3 | 0 | -0.011635 |
| 0 | 1 | 2 | -0.011629 |
| 1 | 0 | 0 | 0.006086 |
| 0 | 0 | 0 | 0.005891 |
| 0 | 0 | 2 | -0.005262 |
| 2 | 0 | 0 | -0.004613 |
| 0 | 2 | 2 | -0.002934 |
| 4 | 1 | 0 | -0.002844 |
| 2 | 1 | 2 | -0.002491 |
| 0 | 3 | 2 | -0.002463 |
| 2 | 2 | 0 | -0.001795 |
| 2 | 3 | 0 | -0.001752 |
| 1 | 4 | 0 | 0.001744 |
| 0 | 1 | 4 | -0.001066 |

$|e_2\rangle$

| K$_1$ | K$_2$ | K$_3$ | $C^{SC}_{2,\boldsymbol{K}}$ |
|---|---|---|---|
| 0 | 2 | 0 | 0.978856 |
| 1 | 0 | 0 | 0.120459 |
| 0 | 3 | 0 | -0.107257 |
| 1 | 2 | 0 | -0.071794 |
| 0 | 4 | 0 | 0.059891 |
| 0 | 1 | 0 | 0.045155 |
| 1 | 1 | 0 | -0.031993 |
| 2 | 0 | 0 | -0.031021 |
| 0 | 5 | 0 | -0.028050 |
| 1 | 4 | 0 | 0.024698 |
| 0 | 2 | 2 | 0.017476 |
| 2 | 2 | 0 | 0.017059 |
| 3 | 2 | 0 | -0.015825 |
| 1 | 2 | 2 | -0.014788 |
| 1 | 3 | 0 | -0.012247 |
| 0 | 0 | 0 | 0.011773 |
| 0 | 1 | 2 | 0.008662 |
| 1 | 5 | 0 | -0.007141 |
| 2 | 1 | 0 | 0.006155 |
| 3 | 0 | 0 | 0.004772 |
| 4 | 0 | 0 | -0.004519 |
| 0 | 6 | 0 | 0.004510 |
| 2 | 4 | 0 | 0.003407 |
| 0 | 3 | 2 | 0.003247 |
| 0 | 4 | 2 | 0.003215 |
| 2 | 0 | 2 | -0.002869 |
| 1 | 0 | 2 | 0.002624 |
| 2 | 2 | 2 | 0.002591 |
| 1 | 6 | 0 | 0.001900 |
| 1 | 1 | 2 | -0.001860 |
| 2 | 5 | 0 | -0.001796 |
| 4 | 2 | 0 | 0.001487 |
| 0 | 2 | 4 | 0.001379 |
| 3 | 3 | 0 | 0.001343 |
| 2 | 6 | 0 | 0.001114 |

$|e_3\rangle$

| K$_1$ | K$_2$ | K$_3$ | $C^{SC}_{3,\boldsymbol{K}}$ |
|---|---|---|---|
| 1 | 0 | 0 | 0.910605 |
| 2 | 0 | 0 | -0.339461 |
| 0 | 0 | 0 | 0.160178 |
| 0 | 2 | 0 | -0.122539 |
| 3 | 0 | 0 | 0.076325 |
| 4 | 0 | 0 | -0.056048 |
| 0 | 0 | 2 | -0.051814 |
| 1 | 2 | 0 | 0.035378 |
| 2 | 0 | 2 | -0.023173 |
| 1 | 0 | 2 | 0.022954 |
| 5 | 0 | 0 | 0.021571 |
| 1 | 1 | 0 | 0.013387 |
| 3 | 0 | 2 | 0.010423 |
| 6 | 0 | 0 | -0.005492 |
| 3 | 2 | 0 | 0.005342 |
| 0 | 1 | 0 | 0.004997 |
| 2 | 1 | 0 | -0.003580 |
| 2 | 2 | 0 | 0.003232 |
| 4 | 0 | 2 | -0.002829 |
| 1 | 2 | 2 | 0.002680 |
| 1 | 0 | 4 | 0.002574 |
| 0 | 0 | 4 | -0.002488 |
| 1 | 4 | 0 | -0.002351 |
| 7 | 0 | 0 | 0.002254 |
| 4 | 2 | 0 | -0.001982 |
| 1 | 3 | 0 | -0.001914 |
| 3 | 1 | 0 | 0.001778 |
| 0 | 1 | 2 | -0.001629 |
| 1 | 1 | 2 | 0.001612 |
| 0 | 2 | 2 | -0.001578 |
| 5 | 0 | 2 | 0.001322 |
| 2 | 0 | 4 | -0.001086 |
| 2 | 2 | 2 | -0.001026 |

$|e_4\rangle$

| K$_1$ | K$_2$ | K$_3$ | $C^{SC}_{4,\boldsymbol{K}}$ |
|---|---|---|---|
| 0 | 0 | 1 | 0.950271 |
| 0 | 1 | 1 | 0.056333 |
| 0 | 2 | 1 | 0.017098 |
| 1 | 0 | 1 | -0.291333 |
| 1 | 1 | 1 | -0.013388 |
| 1 | 2 | 1 | 0.002040 |
| 2 | 0 | 1 | 0.068064 |
| 0 | 0 | 3 | 0.019709 |
| 2 | 1 | 1 | 0.002551 |
| 0 | 1 | 3 | 0.006701 |
| 0 | 2 | 3 | 0.004479 |
| 3 | 0 | 1 | -0.024522 |
| 1 | 0 | 3 | -0.048320 |
| 3 | 1 | 1 | -0.001152 |
| 1 | 1 | 3 | -0.003678 |
| 1 | 2 | 3 | -0.001345 |
| 4 | 0 | 1 | 0.008717 |
| 2 | 0 | 3 | 0.016934 |
| 0 | 0 | 5 | 0.004325 |
| 5 | 0 | 1 | -0.002471 |
| 3 | 0 | 3 | -0.003855 |
| 1 | 0 | 5 | -0.001709 |
| 4 | 0 | 3 | 0.001228 |
| 2 | 0 | 5 | 0.001665 |

Table S2. The nine largest coefficients in the ground state wavefunction of protonated Glycine.

| $K_1$ | $K_2$ | $K_3$ | $K_4$ | $K_5$ | $K_6$ | $K_7$ | $K_8$ | $K_9$ | $K_{10}$ | $K_{11}$ | $K_{12}$ | $K_{13}$ | $K_{14}$ | $K_{15}$ | $K_{16}$ | $K_{17}$ | $K_{18}$ | $K_{19}$ | $K_{20}$ | $K_{21}$ | $K_{22}$ | $K_{23}$ | $K_{24}$ | $K_{25}$ | $K_{26}$ | $K_{27}$ | $C^{SC}_{0,\boldsymbol{K}}$ |
|---|---|---|---|---|---|---|---|---|---|---|---|---|---|---|---|---|---|---|---|---|---|---|---|---|---|---|---|
| 0 | 0 | 0 | 0 | 0 | 0 | 0 | 0 | 0 | 0 | 0 | 0 | 0 | 0 | 0 | 0 | 0 | 0 | 0 | 0 | 0 | 0 | 0 | 0 | 0 | 0 | 0 | 9,28E-01 |
| 0 | 0 | 0 | 0 | 0 | 0 | 0 | 1 | 0 | 0 | 0 | 0 | 0 | 0 | 0 | 0 | 0 | 0 | 0 | 0 | 0 | 0 | 0 | 0 | 0 | 0 | 0 | 9,82E-02 |
| 0 | 0 | 0 | 0 | 0 | 0 | 0 | 0 | 0 | 0 | 0 | 0 | 0 | 0 | 0 | 0 | 0 | 0 | 0 | 0 | 0 | 1 | 0 | 0 | 0 | 0 | 0 | -8,80E-02 |
| 2 | 0 | 0 | 0 | 0 | 0 | 0 | 0 | 0 | 0 | 0 | 0 | 0 | 0 | 0 | 0 | 0 | 0 | 0 | 0 | 0 | 0 | 0 | 0 | 0 | 0 | 0 | 8,09E-02 |
| 0 | 0 | 1 | 0 | 0 | 0 | 0 | 0 | 0 | 0 | 0 | 0 | 0 | 0 | 0 | 0 | 0 | 0 | 0 | 0 | 0 | 0 | 0 | 0 | 0 | 0 | 0 | -7,68E-02 |
| 0 | 0 | 0 | 0 | 0 | 0 | 0 | 0 | 0 | 0 | 0 | 0 | 0 | 0 | 0 | 0 | 0 | 2 | 0 | 0 | 0 | 0 | 0 | 0 | 0 | 0 | 0 | 6,70E-02 |
| 0 | 0 | 0 | 1 | 0 | 0 | 0 | 0 | 0 | 0 | 0 | 0 | 0 | 0 | 0 | 0 | 0 | 0 | 0 | 0 | 0 | 0 | 0 | 0 | 0 | 0 | 0 | -6,42E-02 |
| 0 | 0 | 0 | 0 | 0 | 0 | 0 | 0 | 0 | 0 | 0 | 0 | 0 | 0 | 0 | 0 | 0 | 0 | 0 | 0 | 0 | 0 | 1 | 0 | 0 | 0 | 0 | 5,31E-02 |
| 2 | 0 | 0 | 0 | 0 | 0 | 0 | 0 | 0 | 0 | 0 | 0 | 0 | 0 | 0 | 0 | 0 | 0 | 0 | 0 | 0 | 0 | 0 | 0 | 1 | 0 | 0 | -4,78E-02 |

Table S3. The fourteen largest coefficients in the $\nu_{23} = 1$ excited state wavefunction of protonated Glycine.

| $K_1$ | $K_2$ | $K_3$ | $K_4$ | $K_5$ | $K_6$ | $K_7$ | $K_8$ | $K_9$ | $K_{10}$ | $K_{11}$ | $K_{12}$ | $K_{13}$ | $K_{14}$ | $K_{15}$ | $K_{16}$ | $K_{17}$ | $K_{18}$ | $K_{19}$ | $K_{20}$ | $K_{21}$ | $K_{22}$ | $K_{23}$ | $K_{24}$ | $K_{25}$ | $K_{26}$ | $K_{27}$ | $C^{SC}_{23,\boldsymbol{K}}$ |
|---|---|---|---|---|---|---|---|---|---|---|---|---|---|---|---|---|---|---|---|---|---|---|---|---|---|---|---|
| 0 | 0 | 0 | 0 | 0 | 0 | 0 | 0 | 0 | 0 | 0 | 0 | 0 | 1 | 0 | 0 | 0 | 0 | 0 | 1 | 0 | 0 | 0 | 0 | 0 | 0 | 0 | 3,66E-01 |
| 0 | 0 | 0 | 0 | 0 | 0 | 0 | 0 | 0 | 0 | 0 | 0 | 0 | 0 | 0 | 0 | 0 | 0 | 0 | 0 | 0 | 0 | 1 | 0 | 0 | 0 | 0 | 3,56E-01 |
| 0 | 0 | 0 | 0 | 0 | 0 | 0 | 0 | 0 | 0 | 0 | 0 | 0 | 0 | 0 | 0 | 2 | 0 | 0 | 0 | 0 | 0 | 0 | 0 | 0 | 0 | 0 | -3,38E-01 |
| 0 | 0 | 0 | 0 | 0 | 0 | 0 | 0 | 0 | 0 | 0 | 0 | 0 | 0 | 0 | 0 | 0 | 0 | 0 | 0 | 0 | 1 | 0 | 0 | 0 | 0 | 0 | 2,04E-01 |
| 1 | 0 | 0 | 0 | 0 | 0 | 0 | 0 | 0 | 0 | 0 | 0 | 0 | 0 | 0 | 0 | 0 | 0 | 0 | 0 | 0 | 0 | 0 | 1 | 0 | 0 | 0 | 1,75E-01 |
| 0 | 0 | 0 | 0 | 0 | 0 | 0 | 0 | 2 | 0 | 1 | 0 | 0 | 0 | 0 | 0 | 0 | 0 | 0 | 0 | 0 | 0 | 0 | 0 | 0 | 0 | 0 | 1,42E-01 |
| 0 | 0 | 0 | 0 | 0 | 0 | 0 | 0 | 0 | 0 | 1 | 0 | 0 | 0 | 0 | 0 | 0 | 0 | 0 | 0 | 1 | 0 | 0 | 0 | 0 | 0 | 0 | 1,41E-01 |
| 0 | 0 | 0 | 0 | 2 | 0 | 0 | 0 | 2 | 0 | 0 | 0 | 0 | 0 | 0 | 0 | 0 | 0 | 0 | 0 | 0 | 0 | 0 | 0 | 0 | 0 | 0 | 1,35E-01 |
| 0 | 0 | 0 | 1 | 0 | 0 | 0 | 0 | 0 | 0 | 0 | 0 | 2 | 0 | 0 | 0 | 0 | 0 | 0 | 0 | 0 | 0 | 0 | 0 | 0 | 0 | 0 | -1,27E-01 |
| 0 | 0 | 0 | 0 | 0 | 0 | 0 | 0 | 0 | 0 | 0 | 0 | 0 | 0 | 1 | 0 | 1 | 0 | 0 | 0 | 0 | 0 | 0 | 0 | 0 | 0 | 0 | -1,19E-01 |
| 0 | 0 | 0 | 0 | 0 | 0 | 0 | 0 | 2 | 0 | 0 | 0 | 0 | 0 | 1 | 0 | 0 | 0 | 0 | 0 | 0 | 0 | 0 | 0 | 0 | 0 | 0 | -1,12E-01 |
| 0 | 0 | 1 | 0 | 0 | 0 | 0 | 0 | 0 | 0 | 0 | 0 | 0 | 0 | 2 | 0 | 0 | 0 | 0 | 0 | 0 | 0 | 0 | 0 | 0 | 0 | 0 | 1,12E-01 |
| 0 | 0 | 0 | 0 | 4 | 0 | 0 | 1 | 0 | 0 | 0 | 0 | 0 | 0 | 0 | 0 | 0 | 0 | 0 | 0 | 0 | 0 | 0 | 0 | 0 | 0 | 0 | 1,08E-01 |
| 0 | 0 | 0 | 0 | 0 | 0 | 0 | 0 | 0 | 0 | 0 | 0 | 0 | 0 | 1 | 0 | 0 | 0 | 1 | 0 | 0 | 0 | 0 | 0 | 0 | 0 | 0 | -1,07E-01 |

## II. EXPANSION COEFFICIENTS FOR PROTONATED GLYCINE EIGENFUNCTIONS

Table S4. The eleven largest coefficients in the $\nu_{25} = 1$ excited state wavefunction of protonated Glycine.

| $K_1$ | $K_2$ | $K_3$ | $K_4$ | $K_5$ | $K_6$ | $K_7$ | $K_8$ | $K_9$ | $K_{10}$ | $K_{11}$ | $K_{12}$ | $K_{13}$ | $K_{14}$ | $K_{15}$ | $K_{16}$ | $K_{17}$ | $K_{18}$ | $K_{19}$ | $K_{20}$ | $K_{21}$ | $K_{22}$ | $K_{23}$ | $K_{24}$ | $K_{25}$ | $K_{26}$ | $K_{27}$ | $C^{SC}_{25,\boldsymbol{K}}$ |
|---|---|---|---|---|---|---|---|---|---|---|---|---|---|---|---|---|---|---|---|---|---|---|---|---|---|---|---|
| 0 | 0 | 1 | 0 | 0 | 0 | 0 | 0 | 0 | 0 | 0 | 0 | 0 | 0 | 0 | 0 | 0 | 0 | 0 | 0 | 0 | 0 | 1 | 0 | 0 | 0 | 0 | 3,77E-01 |
| 0 | 0 | 0 | 0 | 0 | 0 | 0 | 1 | 0 | 0 | 0 | 0 | 0 | 2 | 0 | 0 | 0 | 0 | 0 | 0 | 0 | 0 | 0 | 0 | 0 | 0 | 0 | 3,69E-01 |
| 0 | 0 | 0 | 0 | 0 | 0 | 0 | 0 | 0 | 0 | 0 | 0 | 0 | 0 | 0 | 0 | 0 | 0 | 0 | 0 | 0 | 0 | 0 | 0 | 1 | 0 | 0 | 3,67E-01 |
| 0 | 0 | 1 | 0 | 0 | 0 | 0 | 0 | 0 | 0 | 0 | 0 | 0 | 0 | 0 | 0 | 0 | 0 | 0 | 0 | 0 | 1 | 0 | 0 | 0 | 0 | 0 | 2,00E-01 |
| 0 | 0 | 0 | 0 | 0 | 0 | 0 | 0 | 0 | 0 | 0 | 0 | 0 | 0 | 0 | 0 | 0 | 1 | 0 | 0 | 1 | 0 | 0 | 0 | 0 | 0 | 0 | -1,76E-01 |
| 0 | 0 | 0 | 1 | 0 | 0 | 0 | 0 | 0 | 0 | 0 | 0 | 0 | 0 | 0 | 0 | 0 | 2 | 0 | 0 | 0 | 0 | 0 | 0 | 0 | 0 | 0 | 1,72E-01 |
| 0 | 1 | 0 | 0 | 0 | 0 | 0 | 0 | 0 | 0 | 0 | 0 | 0 | 0 | 0 | 0 | 0 | 0 | 0 | 0 | 0 | 0 | 0 | 1 | 0 | 0 | 0 | 1,59E-01 |
| 1 | 0 | 0 | 0 | 0 | 0 | 0 | 0 | 0 | 0 | 0 | 0 | 0 | 0 | 0 | 0 | 0 | 0 | 0 | 0 | 0 | 0 | 0 | 1 | 0 | 0 | 0 | -1,32E-01 |
| 0 | 0 | 0 | 0 | 0 | 0 | 0 | 0 | 2 | 0 | 0 | 0 | 0 | 0 | 0 | 0 | 0 | 1 | 0 | 0 | 0 | 0 | 0 | 0 | 0 | 0 | 0 | -1,26E-01 |
| 0 | 0 | 0 | 0 | 0 | 0 | 0 | 0 | 0 | 2 | 0 | 0 | 0 | 0 | 0 | 1 | 0 | 0 | 0 | 0 | 0 | 0 | 0 | 0 | 0 | 0 | 0 | -1,19E-01 |
| 0 | 0 | 0 | 0 | 0 | 0 | 0 | 0 | 0 | 2 | 0 | 0 | 0 | 0 | 0 | 0 | 1 | 0 | 0 | 0 | 0 | 0 | 0 | 0 | 0 | 0 | 0 | -1,12E-01 |

Table S5. The eleven largest coefficients in the $\nu_{26} = 1$ excited state wavefunction of protonated Glycine.

| $K_1$ | $K_2$ | $K_3$ | $K_4$ | $K_5$ | $K_6$ | $K_7$ | $K_8$ | $K_9$ | $K_{10}$ | $K_{11}$ | $K_{12}$ | $K_{13}$ | $K_{14}$ | $K_{15}$ | $K_{16}$ | $K_{17}$ | $K_{18}$ | $K_{19}$ | $K_{20}$ | $K_{21}$ | $K_{22}$ | $K_{23}$ | $K_{24}$ | $K_{25}$ | $K_{26}$ | $K_{27}$ | $C^{SC}_{26,\boldsymbol{K}}$ |
|---|---|---|---|---|---|---|---|---|---|---|---|---|---|---|---|---|---|---|---|---|---|---|---|---|---|---|---|
| 0 | 0 | 0 | 0 | 0 | 0 | 0 | 0 | 0 | 0 | 0 | 0 | 0 | 0 | 0 | 0 | 0 | 0 | 0 | 0 | 0 | 0 | 0 | 0 | 0 | 1 | 0 | 6,95E-01 |
| 0 | 0 | 0 | 0 | 1 | 0 | 0 | 0 | 0 | 0 | 0 | 0 | 0 | 0 | 0 | 0 | 0 | 2 | 0 | 0 | 0 | 0 | 0 | 0 | 0 | 0 | 0 | 4,18E-01 |
| 0 | 0 | 1 | 0 | 0 | 0 | 0 | 0 | 0 | 0 | 0 | 0 | 0 | 0 | 0 | 0 | 0 | 0 | 0 | 0 | 0 | 0 | 0 | 1 | 0 | 0 | 0 | -2,73E-01 |
| 0 | 0 | 0 | 0 | 0 | 0 | 0 | 0 | 0 | 0 | 0 | 0 | 0 | 0 | 0 | 0 | 0 | 0 | 0 | 0 | 0 | 0 | 0 | 0 | 1 | 1 | 0 | 9,36E-02 |
| 1 | 0 | 0 | 0 | 0 | 0 | 0 | 0 | 0 | 0 | 0 | 0 | 0 | 0 | 0 | 0 | 0 | 0 | 0 | 0 | 0 | 0 | 0 | 0 | 1 | 0 | 0 | 9,28E-02 |
| 0 | 0 | 0 | 0 | 0 | 0 | 0 | 0 | 0 | 0 | 0 | 2 | 0 | 1 | 0 | 0 | 0 | 0 | 0 | 0 | 0 | 0 | 0 | 0 | 0 | 0 | 0 | 9,20E-02 |
| 0 | 0 | 0 | 0 | 0 | 0 | 0 | 1 | 0 | 0 | 0 | 0 | 0 | 0 | 0 | 0 | 0 | 0 | 0 | 0 | 0 | 0 | 0 | 0 | 0 | 1 | 0 | 9,05E-02 |
| 0 | 0 | 0 | 0 | 0 | 0 | 0 | 0 | 0 | 0 | 2 | 0 | 0 | 1 | 0 | 0 | 0 | 0 | 0 | 0 | 0 | 0 | 0 | 0 | 0 | 0 | 0 | 8,67E-02 |
| 0 | 0 | 0 | 1 | 0 | 0 | 0 | 0 | 0 | 0 | 0 | 0 | 0 | 0 | 0 | 0 | 0 | 0 | 0 | 0 | 0 | 0 | 0 | 0 | 0 | 1 | 0 | 8,39E-02 |
| 0 | 0 | 0 | 0 | 0 | 0 | 0 | 0 | 0 | 0 | 0 | 0 | 0 | 0 | 0 | 0 | 0 | 0 | 0 | 1 | 1 | 0 | 0 | 0 | 0 | 0 | 0 | -8,34E-02 |
| 2 | 0 | 0 | 0 | 0 | 0 | 0 | 0 | 0 | 0 | 0 | 0 | 0 | 0 | 0 | 0 | 0 | 0 | 0 | 0 | 0 | 0 | 0 | 1 | 0 | 0 | 0 | -8,00E-02 |

## III. ADDITIONAL PLOTS OF RELEVANT BOND-LENGTH, ANGLE AND DIHEDRAL DISTRIBUTIONS FOR PROTONATED GLYCINE MOLECULE

### A. $\nu_{23} = 1$ state

#### *1. Angle distributions*

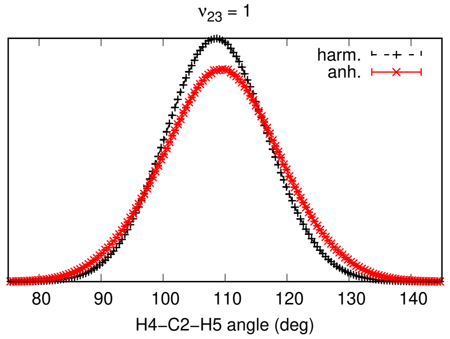


Figure S1.

#### *2. Bond-length distributions*

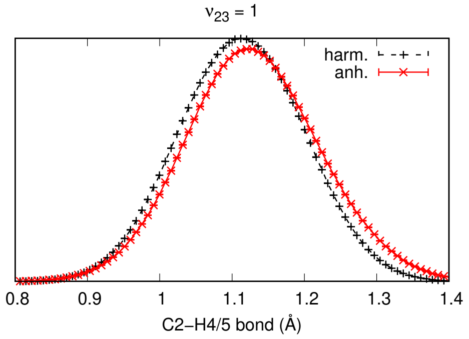


Figure S2.

### *3. Dihedral distributions*

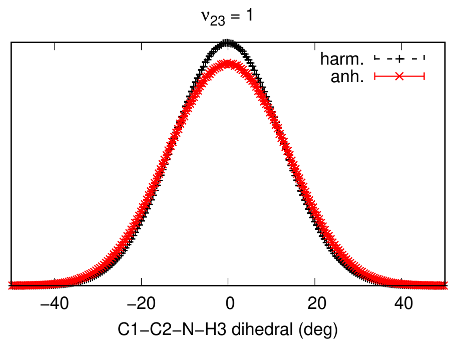


Figure S3.

## B. $\nu_{25} = 1$ state

### *1. Angle distributions*

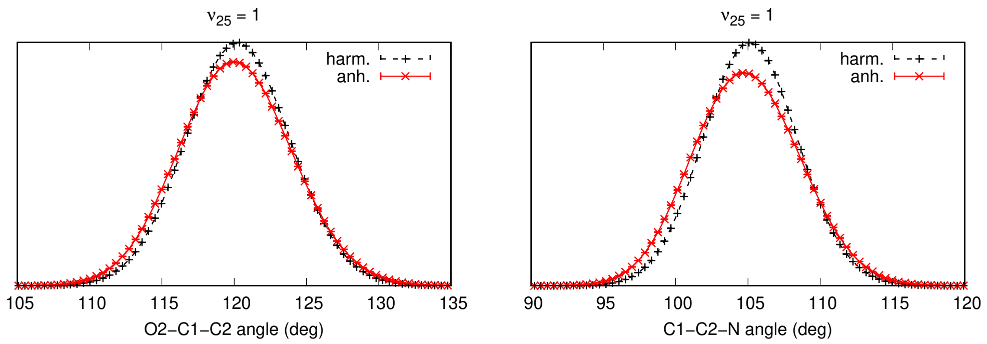


Figure S4.

### *2. Bond-length distributions*

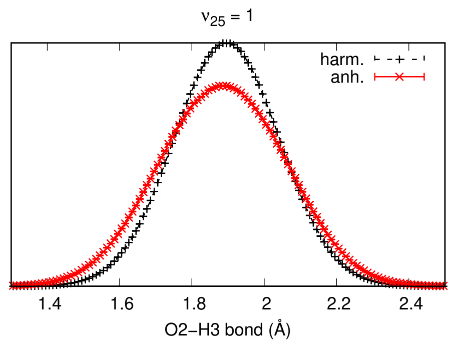


Figure S5.

### 3. *Dihedral distributions*

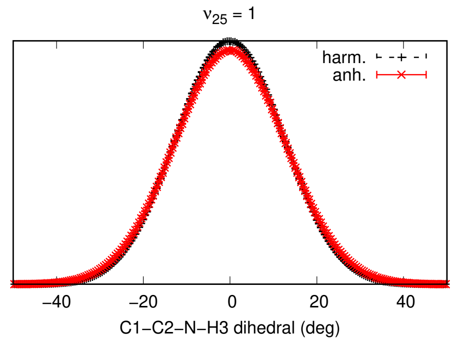


Figure S6.

## C. $\nu_{26} = 1$ state

### 1. *Angle distributions*

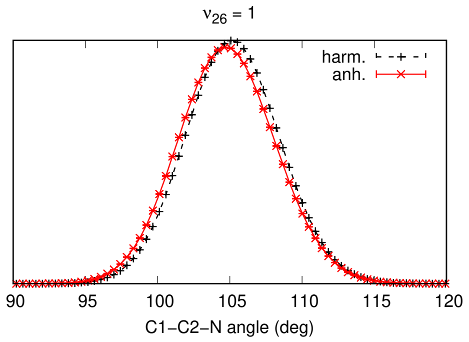


Figure S7.

### 2. *Bond-length distributions*

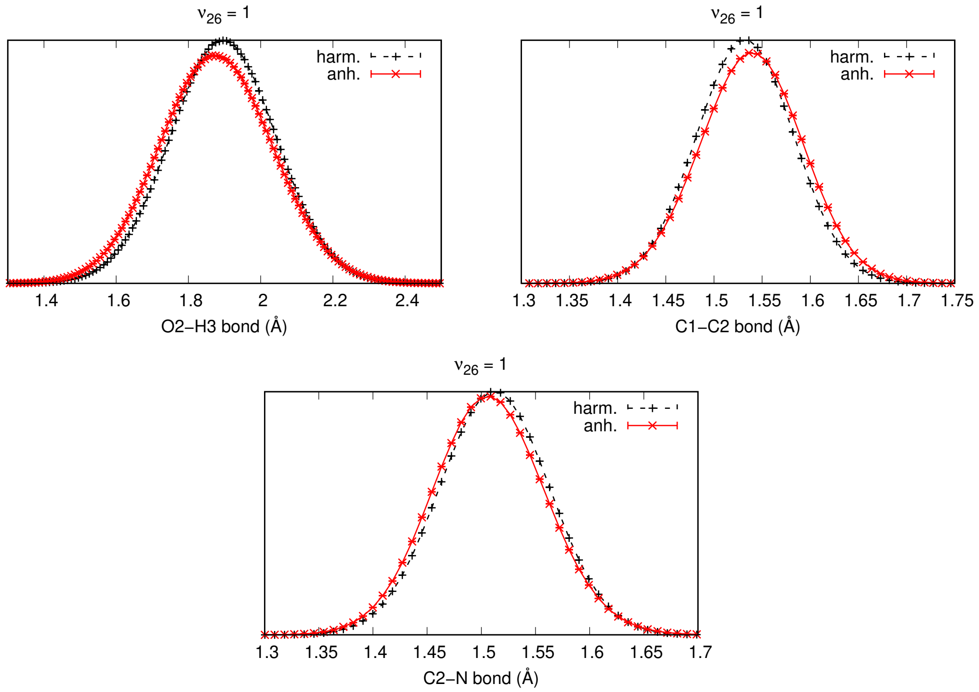


Figure S8.

### 3. *Dihedral distributions*

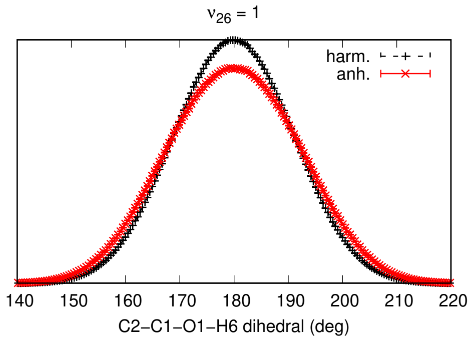


Figure S9.
